# Supplementary material for: The Dark Energy Survey Six-Year Calibration Star Catalog
Source: arXiv:2305.01695 source file (2023-05-02)
Supplement: Supplementary file 1 [file appendix.tex]

\appendix
\numberwithin{figure}{section}
\numberwithin{table}{section}

\section{Weight average quantities}
\label{app:wavg}

The weighted-average (\var{WAVG}) quantities are derived from the individual single-epoch \SExtractor measurements for all detections of the same object in a given band that pass the following selection criteria:  
(1) $\var{FLAGS} < 4$ (i.e., allow blends and neighbors, but not saturated detections) 
(2) $\var{IMAFLAGS\_ISO}=0$ (i.e., remove detections that overlap a CCD defect such as a bad column, a cosmic ray or a stellar bleed trail).  
(3) \var{MAG\_PSF} < 99 (i.e., require the detection has a valid \var{MAG\_PSF} measurement in a single-epoch image). 
The \var{NEPOCH} variable tracks the number of detections that pass these selection criteria and are used to calculate the \var{WAVG} quantities.
There are many faint objects that are only detected in the coadded images, and thus have \var{NEPOCH} = 0 and no valid \var{WAVG} measurements in one or more bands.

%Detections of single-epoch objects which pass the selections described above are included in a \var{NEPOCH} count of the number of good detections of the object, and only these conservative detections go into the weighted average \var{WAVG\_MAG\_PSF} magnitude.

%Because the object must be detected in a single-epoch image to increment the \var{NEPOCH} counter for that object in that band, 

We calculate the \var{WAVG\_MAG\_PSF} from the individual \var{MAG\_PSF} measurements, $i$, in a given band as:
\begin{equation}
    \var{WAVG\_MAG\_PSF} = \frac{\sum_{i=1}^{i=\var{NEPOCH}} (\var{MAG\_PSF}_{i} \times w_{i}) }{ \sum_{i=1}^{i=\var{NEPOCH}} w_{i}} \ .
\end{equation} 
Each measurement is weighted by a factor:
\begin{equation}
w_{i} = ( (\var{MAGERR\_PSF})^2 + (0.001)^2 )^{-1} \ .
\end{equation}  
The constant term 0.001 is an `error floor' determined empirically to avoid underestimating the errors on very bright objects. The error on the \var{WAVG\_MAG\_PSF} quantity is calculated as 
\begin{equation}
    \var{WAVG\_MAGERR\_PSF} = \frac{\sqrt{\sum_{i=1}^{i=\var{NEPOCH}}(\var{MAGERR\_PSF}_{i})^2}}{\var{NEPOCH}}
\end{equation} 
and is a simple measure of the spread in errors for individual detections of a given object in a given band. Similar formulae apply for the calculation of the \var{WAVG\_SPREAD\_MODEL} and \var{WAVG\_SPREADERR\_MODEL} quantities, which are derived from the individual single-epoch \var{SPREAD\_MODEL} measurements with an error floor of $10^{-6}$.
We note that the use of \var{WAVG\_MAG\_PSF} is only recommended for point-like sources.

These definitions of the weighted average (including an error floor) and the error on the average are somewhat non-standard, and have not been robustly verified near the detection limit using fluxes instead of magnitude quantities. However, for stellar objects down to $g \sim 23$, they represent a robust determination of a combined magnitude, which has been used in the past for work on resolved stellar populations and photometric calibration. The main advantage of the \var{WAVG\_MAG\_PSF} quantities for stellar work is that the PSF model is fit on each single-epoch image rather than the coadded image. This makes the \var{WAVG} quantities for bright point-like sources more accurate than those derived from the deeper coadded images.

Precise cosmological analyses with DES utilize magnitudes and morphological parameters derived from simultaneous fitting of the single-epoch images \citep[e.g., the \var{SOF} quantities;][]{Y1A1,Y3Gold}. 
These measurements do not suffer from the depth limitations of the \var{WAVG} magnitudes, which are derived from independent single-epoch images. 
We expected that the simultaneously fit quantities derived from the DES DR2 data will be released in support of the DES cosmology analyses in future instances of the DES `Gold' catalog.

\section{Photometric Transformations}
\label{app:transform}

Here, we provide empirical photometric transformations between DES and several other current and recent sky surveys.

We note that transformation equations can have many forms and are generally dependent on the types of objects for which the photometry is being transformed.  Here, we have striven for relatively simple equations based on stars of relatively typical color.  As such, these equations should work reasonably well for objects with SEDs not too dissimilar to ``normal'' stars, but less so for other objects (e.g., objects with strong emission lines).
Quality plots and any future updates for these transformations can be found on the DES DR2 webpage.\footnote{\url{https://des.ncsa.illinois.edu/releases/dr2}}

\subsection{SDSS}

Here, we matched stars from DES DR2 to stars in the Stripe 82 area of SDSS DR13~\citep{dr13}, using the \var{WAVG\_PSF\_MAG}'s from DES and the \var{PSF\_MAG}'s from SDSS.  To reduce the effects of photon noise, we only considered stars with rms magnitude errors of $\leq$0.01 in DES and $\leq$0.02 in SDSS. For outlier rejection, we made use of iterated sigma-clipping, iterating over the fit 3$\times$ and removing 3$\sigma$ outliers after each iteration. Finally we found:
\begin{equation}
\begin{aligned}
g_{\rm DES} = g_{\rm SDSS} - 0.061 (g - i)_{\rm SDSS} + 0.008 ~(RMS:  0.017~\rm{mag})\\
r_{\rm DES} = r_{\rm SDSS} - 0.155 (r - i)_{\rm SDSS} - 0.007 ~(RMS:  0.014~\rm{mag})\\
i_{\rm DES} = i_{\rm SDSS} - 0.166 (r - i)_{\rm SDSS} + 0.032 ~(RMS:  0.018~\rm{mag})\\
z_{\rm DES} = z_{\rm SDSS} - 0.056 (r - i)_{\rm SDSS} + 0.027 ~(RMS:  0.018~\rm{mag})
\end{aligned}
\end{equation}
\begin{equation}
\begin{aligned}
g_{\rm SDSS} = g_{\rm DES} + 0.060 (g - i)_{\rm DES} - 0.005 ~(RMS:  0.018~\rm{mag})\\
r_{\rm SDSS} = r_{\rm DES} + 0.150 (r - i)_{\rm DES} + 0.014 ~(RMS:  0.016~\rm{mag})\\
i_{\rm SDSS} = i_{\rm DES} + 0.167 (r - i)_{\rm DES} - 0.027 ~(RMS:  0.015~\rm{mag})\\
z_{\rm SDSS} = z_{\rm DES} + 0.054 (r - i)_{\rm DES} - 0.024 ~(RMS:  0.018~\rm{mag})
\end{aligned}
\end{equation}
-- i.e., first-order polynomials based on a single color index ($g-i$ for $g$ and $r-i$ for $r,i,z$).  These equations are valid for stars with $-1.0 \lesssim g-i \lesssim 3.5$ ($g$) and $-0.4 \lesssim r-i \lesssim 2.0$ ($r,i,z$).  (Note: the $RMS$ listed after each transformation is $RMS$ per star.  The mean $RMS$ for a collection of stars being transformed from one photometric system to the other -- especially if that collection of stars covers a range of colors -- should be correspondingly smaller,  $\sim RMS/\sqrt{N_{\rm stars}}$.)

\subsection{Pan-STARRS}

As for the DES/SDSS transformation equations, here, we matched stars from DES DR2 to stars in the Stripe 82 area of PanSTARRS1 DR2~\citep{panstarsurveys,panstarrsdata}, using the \var{WAVG\_PSF\_MAG}'s from DES and the \var{MeanPSFMag}'s from PanSTARRS1.  Again, to reduce the effects of photon noise, we only considered stars with rms magnitude errors of $\leq$0.01 in DES and $\leq$0.02 in PanSTARRS1.   Using the same type of outlier rejection and aiming for similar goals in accuracy, simplicity, and color coverage, we arrived at the following equations:
\begin{equation}
\begin{aligned}
g_{\rm DES} = g_{\rm PS1} + 0.028 (g - i)_{\rm PS1} + 0.020 ~(RMS:  0.017~\rm{mag})\\
r_{\rm DES} = r_{\rm PS1} - 0.142 (r - i)_{\rm PS1} - 0.010 ~(RMS:  0.013~\rm{mag})\\
i_{\rm DES} = i_{\rm PS1} - 0.155 (r - i)_{\rm PS1} + 0.015 ~(RMS:  0.012~\rm{mag})\\
z_{\rm DES} = z_{\rm PS1} - 0.114 (r - i)_{\rm PS1} - 0.010 ~(RMS:  0.015~\rm{mag})\\
Y_{\rm DES} = y_{\rm PS1} - 0.031 (r - i)_{\rm PS1} + 0.035 ~(RMS:  0.017~\rm{mag})
\end{aligned}
\end{equation}
\begin{equation}
\begin{aligned}
g_{\rm PS1} = g_{\rm DES} - 0.026 (g - i)_{\rm DES} - 0.020 ~(RMS:  0.017~\rm{mag})\\
r_{\rm PS1} = r_{\rm DES} + 0.139 (r - i)_{\rm DES} + 0.014 ~(RMS:  0.015~\rm{mag})\\
i_{\rm PS1} = i_{\rm DES} + 0.153 (r - i)_{\rm DES} - 0.011 ~(RMS:  0.010~\rm{mag})\\
z_{\rm PS1} = z_{\rm DES} + 0.112 (r - i)_{\rm DES} + 0.013 ~(RMS:  0.015~\rm{mag})\\
y_{\rm PS1} = Y_{\rm DES} + 0.031 (r - i)_{\rm DES} - 0.034 ~(RMS:  0.017~\rm{mag})
\end{aligned}
\end{equation}
-- which are valid for stars with $-0.9 \lesssim g-i \lesssim 3.8$ ($g$) and $-0.4 \lesssim r-i \lesssim 2.7$ ($r,i,z,Y$).

\subsection{HSC}

As described in \secref{depth}, we used HSC-PDR2 \citep{HSCPDR2} to report our detection efficiency as a function of DES \var{MAG\_AUTO}. In order to be comparable, transformation equations were derived for \var{MAG\_AUTO} from matched stars between both surveys for high signal-to-noise high confidence stars ($18 < g, r, i < 21$) and with $0.2 < g-r < 1.2$ for all bands. We also removed  2$\sigma$ outliers after a first fit iteration.

\begin{equation}
\begin{aligned}
g_{\rm DES} = g_{\rm HSC}  - 0.012 (g - r)_{\rm HSC} + 0.029~(RMS:  0.027~\rm{mag}) \\
r_{\rm DES} = r_{\rm HSC}  - 0.075 (g - r)_{\rm HSC} + 0.031~(RMS:  0.030~\rm{mag}) \\
i_{\rm DES} = i_{\rm HSC}  - 0.170 (i - z)_{\rm HSC} + 0.022~(RMS:  0.026~\rm{mag}) \\
z_{\rm DES} = z_{\rm HSC}  - 0.081 (i - z)_{\rm HSC} + 0.023~(RMS:  0.033~\rm{mag}) \\
Y_{\rm DES} = Y_{\rm HSC}  + 0.011 (i - z)_{\rm HSC} + 0.077~(RMS:  0.057~\rm{mag})
\end{aligned}
\end{equation}

\subsection{CFHTLenS}

In DR1, DES detection efficiency was assessed against CFHTLens data \citep{2013MNRAS.433.2545E}. For completeness, we also present here the photometric transformations from CFHTLenS to the DES DR2 photometry. Similarly to what was done with HSC-PDR2, transformation equations were derived for \var{MAG\_AUTO} from matched stars between both surveys for high signal-to-noise high confidence stars ($18 < g, r,i < 21$) with $0.2 < g-r < 1.2$ and 2$\sigma$ outliers removed from fit.

\begin{equation}
\begin{aligned}
g_{\rm DES} = g_{\rm CFHTLenS}  + 0.019 (g - r)_{\rm CFHTLenS} + 0.117~(RMS: 0.035~\rm{mag}) \\
r_{\rm DES} = r_{\rm CFHTLenS}  - 0.062 (g - r)_{\rm CFHTLenS} + 0.073~(RMS: 0.025~\rm{mag}) \\
i_{\rm DES} = i_{\rm CFHTLenS}  - 0.142 (i - z)_{\rm CFHTLenS} + 0.099~(RMS: 0.029~\rm{mag}) \\
z_{\rm DES} = z_{\rm CFHTLenS}  + 0.002 (i - z)_{\rm CFHTLenS} + 0.099~(RMS: 0.038~\rm{mag})
\end{aligned}
\end{equation}

\subsection{Johnson-Cousins}

Fitting transformation equations between the DES and the Johnson-Cousins ($UBVR_cIc$) system includes some additional complications.  One complication is that the two photometric
systems are sufficiently different that the $\Delta$mag vs.\ color plots used for the fits start to have the appearance of full-blown color-magnitude diagrams -- with large discontinuities and occasional bifurcations in the stellar locus.  To address this problem, we fit over 2 or 3 piece-wise discontinuous regions along the color axis and try to avoid band/color combinations that show noticeable bifurcations.   The second complication is identifying a large, publicly accessible sample of well-calibrated faint ($V\gtrsim16$) stellar photometry for the Johnson-Cousins system that overlaps the DES DR2 footprint.  We solved this by making use of Peter Stetson's database of Johnson-Cousins standard stars \citep{2009IAUS..258..197S,2019MNRAS.485.3042S}.\footnote{\url{https://www.canfar.net/storage/list/STETSON/Standards}} We note that Stetson's photometry is calibrated to the photometric system defined by \citet{1992AJ....104..340L} and is zeropointed to the {\em Vega\/} system rather than the {\em AB\/} system.
Other than these complications, the process was very similar to fitting the other transformation equations in this section.   We matched stars from DES DR2 to stars in the Stetson database, using the \var{WAVG\_PSF\_MAG}'s from DES and the mean magnitudes from Stetson.  To reduce the effects of photon noise, we only considered stars with rms magnitude errors of $\leq$0.02 in either DES or the Stetson sample, and we only included Stetson stars that had at least 5 observations each in $B$, $V$, $R$, $I$.  These cuts left us with $\approx$10,000 matches.  As before, for outlier rejection, we made use of iterated sigma-clipping, iterating over the fit 3$\times$ and removing 3$\sigma$ outliers after each iteration.  Here are the results:

\begin{eqnarray}
\begin{aligned}
g_{\rm DES} & = & V + 0.552 (B-V) - 0.099 & ~~~~[-0.2 < (B-V) \leq 0.4]       &   ~(RMS:  0.012~\rm{mag})\\
            & = & V + 0.493 (B-V) - 0.067 & ~~~~[0.4 < (B-V) \leq 2.2]        &   ~(RMS:  0.021~\rm{mag})\\
            &   & & & \\
r_{\rm DES} & = & R_c + 0.046 (R-I)_c + 0.160 & ~~~~[-0.2 < (R-I)_c \leq 0.7] &   ~(RMS:  0.015~\rm{mag})\\
            & = & R_c + 0.127 (R-I)_c + 0.113 & ~~~~[0.7 < (R-I)_c \leq 2.0]  &   ~(RMS:  0.021~\rm{mag})\\
            &   & & & \\
i_{\rm DES} & = & I_c + 0.083 (R-I)_c + 0.392 & ~~~~[-0.2 < (R-I)_c \leq 0.7] &   ~(RMS:  0.012~\rm{mag})\\
            & = & I_c + 0.049 (R-I)_c + 0.416 & ~~~~[0.7 < (R-I)_c \leq 2.0]  &   ~(RMS:  0.015~\rm{mag})\\
            &   & & & \\
z_{\rm DES} & = & I_c - 0.546 (R-I)_c + 0.494 & ~~~~[-0.2 < (R-I)_c \leq 0.2] &   ~(RMS:  0.044~\rm{mag})\\
            & = & I_c - 0.546 (R-I)_c + 0.574 & ~~~~[0.2 < (R-I)_c \leq 0.7]  &   ~(RMS:  0.020~\rm{mag})\\
            & = & I_c - 0.341 (R-I)_c + 0.446 & ~~~~[0.7 < (R-I)_c \leq 2.0]  &   ~(RMS:  0.023~\rm{mag})\\
            &   & & & \\
Y_{\rm DES} & = & I_c - 0.818 (R-I)_c + 0.588 & ~~~~[-0.2 < (R-I)_c \leq 0.2] &   ~(RMS:  0.051~\rm{mag})\\
            & = & I_c - 0.831 (R-I)_c + 0.698 & ~~~~[0.2 < (R-I)_c \leq 0.7]  &   ~(RMS:  0.026~\rm{mag})\\
            & = & I_c - 0.437 (R-I)_c + 0.451 & ~~~~[0.7 < (R-I)_c \leq 2.0]  &   ~(RMS:  0.030~\rm{mag})\\
            &   & & & \\
\end{aligned}
\end{eqnarray}

\begin{eqnarray}
\begin{aligned}
B   & = & g_{\rm DES} + 0.371 (g-r)_{\rm DES} + 0.197 & ~~~~[-0.5 < (g-r)_{\rm DES} \leq 0.2]  &  ~(RMS:  0.022~\rm{mag})\\
    & = & g_{\rm DES} + 0.542 (g-r)_{\rm DES} + 0.141 & ~~~~[0.2 < (g-r)_{\rm DES} \leq 0.7]   &  ~(RMS:  0.017~\rm{mag})\\
    & = & g_{\rm DES} + 0.454 (g-r)_{\rm DES} + 0.200 & ~~~~[0.7 < (g-r)_{\rm DES} \leq 1.8]   &  ~(RMS:  0.059~\rm{mag})\\
            &   & & & \\
V   & = & g_{\rm DES} - 0.465 (g-r)_{\rm DES} - 0.020 & ~~~~[-0.5 < (g-r)_{\rm DES} \leq 0.2]  &  ~(RMS:  0.012~\rm{mag})\\
    & = & g_{\rm DES} - 0.496 (g-r)_{\rm DES} - 0.015 & ~~~~[0.2 < (g-r)_{\rm DES} \leq 0.7]   &  ~(RMS:  0.011~\rm{mag})\\
    & = & g_{\rm DES} - 0.445 (g-r)_{\rm DES} - 0.062 & ~~~~[0.7 < (g-r)_{\rm DES} \leq 1.8]   &  ~(RMS:  0.024~\rm{mag})\\
            &   & & & \\
R_c & = & r_{\rm DES} - 0.013 (r-i)_{\rm DES} - 0.174 & ~~~~[-0.4 < (r-i)_{\rm DES} \leq 0.1]  &  ~(RMS:  0.015~\rm{mag})\\
    & = & r_{\rm DES} - 0.074 (r-i)_{\rm DES} - 0.165 & ~~~~[0.1 < (r-i)_{\rm DES} \leq 0.5]   &  ~(RMS:  0.013~\rm{mag})\\
    & = & r_{\rm DES} - 0.120 (r-i)_{\rm DES} - 0.149 & ~~~~[0.5 < (r-i)_{\rm DES} \leq 1.8]   &  ~(RMS:  0.021~\rm{mag})\\
            &   & & & \\
I_c & = & i_{\rm DES} - 0.066 (r-i)_{\rm DES} - 0.411 & ~~~~[-0.4 < (r-i)_{\rm DES} \leq 0.1]  &  ~(RMS:  0.014~\rm{mag})\\
    & = & i_{\rm DES} - 0.068 (r-i)_{\rm DES} - 0.416 & ~~~~[0.1 < (r-i)_{\rm DES} \leq 0.5]   &  ~(RMS:  0.013~\rm{mag})\\
    & = & i_{\rm DES} - 0.044 (r-i)_{\rm DES} - 0.430 & ~~~~[0.5 < (r-i)_{\rm DES} \leq 1.8]   &  ~(RMS:  0.016~\rm{mag})\\
            &   & & & \\
\end{aligned}
\end{eqnarray}
Note that each of the 2 or 3 piece-wise branches in these relations are discontinuous; no effort was made to ensure that the value obtained from the red endpoint of one branch would match the value of the blue endpoint of the next branch.  This was done on purpose, due to the minor discontinuities and/or bifurcations seen in the stellar locus of the plotted relations.  We also note that, due to a moderately large bifurcation in the stellar locus, the reddest piece-wise branch ($0.7 < (g-r)_{\rm DES} \leq 1.8$) of the $B \rightarrow g_{\rm DES}$ transformation should be used with some caution (see the quality plots for these relations at the DES DR2 website\footnote{\url{https://des.ncsa.illinois.edu/releases/dr2}}).  Finally, we exclude transformations to/from the Johnson $U$ band, since DES DR2 does not contain DECam $u$-band observations.

\input{appendix_abscalib}

\input{sextractor_flags}

\input{appendix_dr2_tables}

\clearpage
